# Supplementary material for: Mining Sequential Patterns in Uncertain Databases Using Hierarchical Index Structure
Source: arXiv:2404.01347 source file (2024-03-31)
Supplement: Supplementary file 1 [file 00supplementary.tex]

\section*{Motivation}
\label{sec:motivation}
The use of uncertain data in the modern world is increasing day by day. In most of the cases, the database is not static. New increments are added to the database gradually and hence the set of frequent sequences may change. After each increment, running existing algorithms from scratch that can mine frequent sequences in static uncertain databases, is very expensive in terms of time and memory. Therefore it has become inevitable to design an efficient technique that can maintain and update the set of frequent sequences when the database grows incrementally. Few scenarios described below reflect the importance of finding frequent interesting sequences from the incremental uncertain database.

\begin{itemize}
    %\item Will be added soon
    
    \item % \textbf{Scenario 1. Medical Reports: } 
    The novel coronavirus SARS-CoV-2 causes the coronavirus disease of 2019 (COVID-19) which was first seen in China in late 2019. Researchers from the whole world are working on it as the world is expecting to face a huge economic recession with losing a lot of people. If we see the nature of the symptoms of this disease, then it is clear that the symptoms have the nature of the sequential occurrences. Besides, some of the symptoms of this disease are mostly related to other common diseases. So, considering the nature of the symptoms, it can be said that finding weighted frequent sequences of the symptoms of the corona patients can be helpful to predict whether someone is infected or not. Besides, it will be possible to take proper treatment for an infected patient by predicting the next stage of infection based on weighted frequent sequences of symptoms. For example, let at a particular stage of infection, a patient may have mild pain. From the database of symptoms, it has been seen that a patient having mild pain would have serious breathing problems afterward. So it’ll be helpful to take proper precautions for the patient. Moreover, the spreading of the virus is so rapid that we neither can decide from a static database nor find the frequent sequences from scratch every time we get new data. As a consequence, an efficient algorithm to find weighted frequent sequences from incremental databases is very much needed. It can play an important role to determine how the symptoms change with time, how they vary from one region/country to another. Furthermore, so far the technology is not capable enough to give the reports of the patients for the symptoms with precise value. So, the symptoms are measured with some probability values. Let us consider a database of medical reports from coronavirus patients. Each tuple represents reports from an individual patient. For example, $\{(fever: 0.4), (cough: 0.5), (ache\ in\ throat: 0.7, breathing\ problem: 0.9)\}$ may indicate the symptoms of a coronavirus patient. 
    % The database must be dynamic in nature due to the rapid spread of the coronavirus.
    
    %A report is related to one or more symptoms with some order of uncertainty. Moreover, the sequence of the reports is important to diagnose the disease. Besides, not all the symptoms are equally important i.e., they are assigned with different weights. Hence, they are some kind of weighted uncertain sequence data. We may want to mine frequent interesting patterns of symptoms on a weekly or monthly basis. Thus there occurs a sufficient insertion of data which may change the current frequent sequences.
    
    \item % \textbf{Scenario 2. Mining Social Network Data: } 
    Mining social network behavior can be another example of uncertain data. Consider each entry $\{(student: 0.9), (photographer: 0.7, cyclist: 0.3), (tourist: 0.7)\}$ indicates that a particular user is estimated (with some uncertainty) as a student after analyzing his 1st week's behavior, as a photographer or a cyclist after analyzing his 2nd week's behavior and so on. After collecting data of few months from a certain group of users we can find the frequent sequence of behaviors among them. These patterns can be helpful to suggest a user any group, event, customized promotions or offers, etc. After a few months, we collect data about more users and we need to find the updated status of frequent behaviors. Thus the database becomes incremental and challenging.

    \item % \textbf{Scenario 3. Automated Traffic Management System: }
    The traffic management system is being automated to identify vehicles as well as breaking of traffic rules and to analyze the behavior of the drivers. Several methods like Automatic Number Plate Recognition, Speed Recognition, Vehicle Type Recognition, Trajectory Analysis are used which produce uncertain data. We can mine different patterns like ``Going to road A first and then road B is a frequent behavior of 10\% of the cars". These patterns can be helpful in planning and monitoring traffic routes.

\end{itemize}

Few other applications are TNFR (Tumor Necrosis Factor Receptor) disease analysis, DNA sequencing (micro level information with uncertainty), mining in crime data, weather data, fashion trend \cite{rahman2019mining_uWSeq}, and vehicle recognition data \cite{muzammal2011mining_uSeq1st}; WSN (Wireless Sensor Network) data monitoring \cite{zhao2013mining_uncertainSeq}; 
social network behavior analysis \cite{ahmed2016mining} 
etc where a benefit of mining weighted frequent sequential patterns is to discover more meaningful hidden knowledge.

\section*{Proof of lemmas}
\label{sec:proof-of-lemmas}
\begin{lemma}
The \textbf{$expSup^{cap}$} of a sequence is always greater than or equal to the actual expected support of that sequence.
\label{lem:es01}
\end{lemma}

\begin{pf}
To keep the proof less complicated, we consider a sequence $\alpha = <(i_{0})(i_{1})....(i_{m})>$ where each event/itemset consists of a single item, $i_{k}$. \\
% \textbf{Step 1.} Let, $expSup^{Cap}(\alpha) < expSup(\alpha)$ be true.\\
According to the definitions,  $ \forall i_{k} \in \alpha : maxPr(i_{k}) \geq maxPr_{S}(i_{k})$.\\
% Recall that, $\alpha_{k} = <(i_{0})(i_{1})....(i_{k})>$.
% $\Rightarrow \sum_{\forall S \in uSDB} maxPr_{S}(i_{m}) \geq \sum_{\forall S \in uSDB} P_{S_{i}}(i_{m})$
% $\Rightarrow maxPr({\alpha_{m-1}}) \times \sum_{\forall S \in DB} maxPr_{S}(i_{m}) \geq  \sum_{\forall S \in DB} maxPr_{S}(\alpha)$
$\Rightarrow maxPr({i_{0}}) \times \sum_{\forall S \in (DB|{i_{0}})} maxPr_{S}(i_{1}) \geq  \sum_{\forall S \in DB} maxPr_{S}({\textless{}(i_{0})(i_{1})}\textgreater{})$\\
$\Rightarrow maxPr({\alpha_{m-1}}) \times \sum_{\forall S \in (DB|\alpha_{m-1})} maxPr_{S}(i_{m}) \geq  \sum_{\forall S \in DB} maxPr_{S}(\alpha)$\\
$\Rightarrow expSup^{cap}(\alpha) \geq expSup(\alpha)$ \\
$\therefore$ The equality holds only when each item has same existential probability for its all positions in whole database. Otherwise, $expSup^{cap}(\alpha) > expSup(\alpha)$ always be true. \hfill \boxed{}
\end{pf}

\begin{lemma}
For any sequence $\alpha$, the value of $expSup^{cap}(\alpha)$ is always less than or equal to the $expSupport^{top}(\alpha)$ which is used as an upper bound of expected support in uWSequence \cite{rahman2019mining_uWSeq} and can be equivalently defined as $expSupport^{top}(\alpha) = maxPr(\alpha_{m-1})\times maxPr(i_{m}) \times sup_{i_{m}}$ where $sup_{i_{m}}$ denotes the support count of $i_{m}$.
\label{lem:03_capLessTop}
\end{lemma}

\begin{pf} According to definitions,  $\forall S,  \forall i_{k} \in \alpha : maxPr_{S}(i_{k}) \leq maxPr(i_{k})$ 

$\Rightarrow \sum maxPr_{S}(i_{m}) \leq maxPr(i_{m}) \times sup_{i_{m}}$

$\Rightarrow maxPr(\alpha_{m-1}) \times \sum maxPr_{S}(i_{m}) \leq maxPr(\alpha_{m-1}) \times maxPr(i_{m}) \times sup_{i_{m}}$

$\Rightarrow expSup^{cap}(\alpha) \leq expSupport^{top}(\alpha)$
\hfill \boxed{}
\end{pf}

\begin{lemma}
For any sequence $\alpha$, the value of $wgt^{cap}(\alpha)$ is always greater than or equal to the \textit{sWeight} value of its all super sequences.
\label{lem:mw}
\end{lemma}

\begin{pf}
Let us assume that $\alpha  \subset \alpha^{'}$ for some sequence $\alpha^{'}$, 
% $mxW_{S}(\alpha) = mvWgt_{\alpha}$ 
$mxW_{S}(\alpha) \geq sWeight(\alpha)$ from Definition \ref{def:mxw}. \\
The equality holds when the weights of all item in $\alpha$ are equal. Similarly, $mxW_{S}(\alpha^{'}) \geq sWeight(\alpha^{'})$.\\
% Otherwise,
% $mxW_{S}(\alpha) > sWeight(\alpha)$ always holds. \\
% Thus,   it infers that $wgt^{cap}(\alpha)$ can never be lower than the value of $sWeight(\alpha)$. \\
Now, if the weights of all items in database are not equal, then $mxW_{DB}(DB|\alpha) \geq mxW_{DB}(DB|\alpha^{'})$ must hold since $DB|\alpha$ contains all frequent items of $DB|\alpha'$. 
% The item with maximum weight in $\alpha^{'}$ might also be in $\alpha$ or not. \\
Moreover, it is straightforward that $mxW_S(\alpha^{'})$ is always greater than or equal to $mxW_S(\alpha)$. Nevertheless, when $mxW_S(\alpha^{'}) > mxW_S(\alpha)$, the item with maximum weight in $\alpha^{'}$ must come from the projected database, $DB|\alpha$ and thus $mxW_S(\alpha^{'})\leq mxW_{DB}(DB|\alpha)$.\\
$\therefore \max( mxW_S(\alpha^{'}),  mxW_{DB}(DB|\alpha^{'})) \leq \max( mxW_S(\alpha),  mxW_{DB}(DB|\alpha))$\\
$\Rightarrow$ $ wgt^{cap}(\alpha^{'}) \leq wgt^{cap}(\alpha)$ \\
$\Rightarrow  sWeight(\alpha^{'}) \leq wgt^{cap}(\alpha)$ \\
% $\Rightarrow  mvWgt_{\alpha^{'}} \leq wgt^{cap}(\alpha)$ \\
% Thus,  the value of $wgt^{cap}(\alpha)$ will be greater than that of $mvWgt_{\alpha}$. \\ 
Again,  if the weights of all items are equal,  then
$wgt^{cap}(\alpha^{'}) = sWeight(\alpha^{'}) = sWeight(\alpha) = wgt^{cap}(\alpha)$ \\
Therefore,  we can conclude that the value of $wgt^{cap}(\alpha)$ is always greater or equal to the value of $sWeight(\alpha)$ or $sWeight(\alpha^{'})$ which is true for all cases.
\hfill \boxed{}
\end{pf}

\begin{definition}
As we said before, upper bound of weighted expected support is $wExpSup^{cap}(\alpha)$ defined as, 
\begin{equation}
    wExpSup^{cap}(\alpha) = expSup^{cap}(\alpha) \times wgt^{cap}({\alpha})
    \label{eq_wExpSup_cap}
\end{equation}

\end{definition}

\begin{lemma}
\label{lem:wes01}
The value of $wExpSup^{cap}(\alpha)$ is always greater than or equal to actual weighted expected support of a sequence $\alpha$,  $WES(\alpha)$. Hence,  using the $wExpSup^{cap}$ value of any sequence as the upper bound of weighted expected support in mining patterns,  it may generate some false positive frequent patterns.

\end{lemma}
\begin{pf}
Lemma  \ref{lem:es01} and  \ref{lem:mw} has showed that for a sequence $\alpha$, 

$expSup^{cap}(\alpha) \geq expSup(\alpha)$ and $wgt^{cap}(\alpha) \geq sWeight(\alpha)$ \\
$ \Rightarrow  expSup^{cap}(\alpha) \times wgt^{cap}(\alpha) \geq expSup(\alpha) \times sWeight(\alpha) $ \\
$ \Rightarrow  wExpSup^{cap}(\alpha) \geq WES(\alpha) $ \\
$\therefore$ The value of $wExpSup^{cap}(\alpha)$ is always greater than or equal to the value of $WES(\alpha)$ for any sequence $\alpha$. As a result,  some patterns might be introduced as frequent patterns due to its higher value of $wExpSup^{cap}$ being not actually weighted frequent.
\hfill \boxed{}
\end{pf}

\begin{lemma}
\label{lem:wescap}
 If the value of $wExpSup^{cap}$ for a sequence, $\alpha$ is below the minimum weighted expected support threshold \textit{minWES},  the value of \textit{WES} for that sequence and its all super sequences must not satisfy. In other words, the sequence $\alpha$ and its all super sequences must not be frequent if the value of $wExpSup^{cap}(\alpha)$ does not satisfy the threshold. Thus, it does not generate any false negative patterns.
\end{lemma}

\begin{pf}
Assume that $\alpha  \subseteq \alpha^{'}$ for some sequence $\alpha^{'}$.
Recall that, expSup($\alpha$) = $\sum_{\forall S\in DB} maxPr_{S}(\alpha)$ \cite{rahman2019mining_uWSeq}.
By definition, $expSup(\alpha)\geq expSup(\alpha')$.\\
Again,  $expSup^{cap}(\alpha) \geq  expSup(\alpha) \Rightarrow$  $expSup^{cap}(\alpha) \geq  expSup(\alpha')$.\\
Moreover, $wgt^{cap}(\alpha)\geq sWeight(\alpha').$\\
Now, $wExpSup^{cap}(\alpha) = expSup^{cap}(\alpha)\times wgt^{cap}(\alpha) \geq expSup(\alpha')\times sWeight(\alpha') = WES(\alpha')$\\
So, if $wExpSup^{cap}(\alpha) < minWES$ holds, then $WES(\alpha')< minWES$ must hold for any $\alpha'\supseteq\alpha$.\\
Therefore, upper bound, $wExpSup^{cap}$ could be able to find out the complete set of frequent patterns.
\hfill \boxed{}
\end{pf}
\section*{Pseudo-codes of Algorithms}
\label{sec:pseudo-codes}
\subsection{SupCalc}
\label{subsec:supcalc-pseudo-code}
\makeatletter
\renewcommand{\ALG@beginalgorithmic}{\small}
\makeatother
\algrenewcommand{\alglinenumber}{\normalsize}

\makeatletter
\renewcommand{\ALG@beginalgorithmic}{\small }
\makeatother
\algrenewcommand{\alglinenumber}{\small}

\begin{algorithm}[tbh]
\caption{Procedure of SupCalc}
\begin{algorithmic}[1]
\Statex
\Require \textit{DB:} initial database,  \textit{candidateTrie}: stores candidate patterns
\Ensure Calculated weighted expected supports for all patterns %\textit{SFS: } the set of semi-frequent patterns \newline
\Statex
\Procedure{SupCalc}{$DB$,  \textit{candidateTrie}}
\ForAll{${\alpha =  < e1, e2, e3,...,en > } \in {DB}$} \Comment{$e_{k}$ is an itemset/event}
\State $ar \gets\ $the array of size equals to the number of events in $|\alpha| $ which is initialized as 1
\State $wgt\_sum,  itm\_cnt \gets$ 0 and 0 \Comment{$wgt\_sum$ - sum of items' weights and $itm\_cnt$ - their counts in a pattern}
\State TrieTraverse($\alpha$, \textit{null}, \textit{candidateTrie.root},  \textit{ar},  \textit{wgt\_sum},  \textit{itm\_cnt})
\EndFor
\EndProcedure                                                
\Statex 

\Procedure{TrieTraverse}{$\alpha$, \textit{cur\_itmset}, \textit{cur\_node},  \textit{ar},  \textit{wgt\_sum},  \textit{itm\_cnt}}
\ForAll{$ node \in cur\_node.descendents$}
\State $cur\_edge \gets$ edge label between current child \textit{node} and \textit{cur\_node}
\State $cur\_ar \gets$ the array of size \textit{ar} initialized as 0 
\ForAll{ $e_{k} \in \alpha$}
\If{S-Extension Is TRUE}
\State $cur\_itmset \gets cur\_edge$
\If{ $cur\_itmset \in e_{k}$ }
\State mxSup $\gets \max^{k-1}_{i = 1} ar_{i}$
\State $cur\_ar_{k}$ $\gets mxSup \times p_{cur\_edge}$ \Comment{$p_{cur\_edge}$ denotes the existential probability of $cur\_edge$ in $e_{k}$} 
\EndIf
\If{ $cur\_itmset \notin e_{k}$ }
\State $cur\_ar_{k}$ $\gets 0$
\EndIf
\EndIf
\If{I-Extension Is TRUE}
\State $ cur\_itmset \gets (cur\_itmset \cup cur\_edge)$ \Comment{$cur\_itmset$ is extended with $cur\_edge$}
\If{ $cur\_itmset \in e_{k}$ }
\State $cur\_ar_{k}$ $\gets ar_{k} \times p_{cur\_edge}$ \Comment{$p_{cur\_edge}$ denotes the existential probability of $cur\_edge$ in $e_{k}$}  
\EndIf
\If{ $cur\_itmset \notin e_{k}$ }
\State $cur\_ar_{k}$ $\gets 0$
\EndIf
\EndIf

\EndFor
\State $mxSup \gets \max^{|\alpha|}_{i=1} cur\_ar_{i}$
\State $cur\_wgt\_sum \gets wgt\_sum + wgt_{cur\_edge}$ \Comment{$wgt_{cur\_edge}$ denotes the weight of $cur\_edge$}
\State $cur\_itm\_cnt \gets itm\_cnt + 1$
\State $node.WES \gets node.WES + mxSup \times \frac{cur\_wgt\_sum}{cur\_itm\_cnt}$
\State TrieTraverse($\alpha$, \textit{cur\_itmset}, \textit{node},  \textit{cur\_ar},  \textit{cur\_wgt\_sum},  \textit{cur\_itm\_cnt})
\EndFor
\EndProcedure
\Statex
\end{algorithmic}
\label{algo:supcal}
\end{algorithm}

% FUSP
\subsection{FUSP}
\label{subsec:fusp-pseudo-code}
\makeatletter
\renewcommand{\ALG@beginalgorithmic}{\small}
\makeatother
\algrenewcommand{\alglinenumber}{\normalsize}

\makeatletter
\renewcommand{\ALG@beginalgorithmic}{\small }
\makeatother
\algrenewcommand{\alglinenumber}{\small}

\begin{algorithm}[tbh]
\caption{Procedure of \textit{FUWS}}
\begin{algorithmic}[1]
\Statex
\Require \textit{DB:} initial database,  \textit{min\_sup:} support threshold,  \textit{wgtFct:} weight factor%\newline
\Ensure \textit{FS:} set of weighted frequent patterns %\textit{SFS: } the set of semi-frequent patterns \newline
\Statex
\Procedure{FUWS}{$DB$,  \textit{min\_sup},  \textit{wgtFct}}
% \State $minExpSup \gets$  \textit{min\_Sup} $\times uSDBsize$ 
% \State
\State $pDB,  WAM \gets preProcess($DB$)$ 
% \Comment{$\forall S \in (uSDB),  \forall {x} \in S: P^{'}_{{x_{i}}} \gets \max_{j=i}^{|S|} P_{x_{j}}$}
\State $freqItms,  maxPrs,  sWgts \gets Determine(\textit{pDB},  \textit{minWES})$  \Comment{List of frequent items, their \textit{maxPr}, and weights }
\ForAll{${\beta } \in {freqItms}$}
\State $\textit{candidateTrie} \gets FUWSP(DB|{\beta }, \beta,  maxPrs_{\beta }, sWgts_{\beta},  sWgts_{\beta},  1)$ 
\EndFor
\State \textbf{Call} SupCalc(\textit{DB},  \textit{candidateTrie})
% \ForAll{$S \in {uSDB}$}
% % \State $candiTrie.update\_support(S)$ \Comment{ $\forall x: Update Support(x),  x \in candidates $}
% \State Update wExpSup(x) for S where x $\in$ candidates
% \EndFor
% \State $candiTrie.update(\textit{minWES})$ \Comment{$\exists x,   Support(x)<minWES:Delete Node(x)$}
\State FS $\gets$ Remove false positives and find frequent patterns from \textit{candidateTrie}
\EndProcedure                                                
\Statex

\Procedure{FUWSP}{$DB|{\alpha }, \ \alpha, \ maxPr_{\alpha },\ mxW_{\alpha}, \ sWgt_{\alpha}, \ |\alpha|$}
\State $freqItms, \ mxPrs, \ sWgts \gets Determine(DB|{\alpha}, \ \textit{minWES})$ for i-extension and
s-extension from $\alpha$.
\ForAll{$ \beta \in freqItms$}
\State $expSup^{cap}(\alpha \cup \beta) \gets maxPr_{\alpha } \times \sum_{\forall S \in (DB|\alpha)}maxPr_{S}({\beta})$
\State $wgt^{cap}(\alpha \cup \beta) \gets \max(mxW_{\alpha}, sWgts)$ \Comment{\textit{sWgts} - List of frequent items' weights in $DB|{\alpha}$}
\If{$wExpSup^{cap}{(\alpha \cup \beta)} = expSup^{cap}(\alpha \cup \beta) \times wgt^{cap}(\alpha \cup \beta) \geq minWES$}
\State $maxPr_{\alpha \cup \beta} \gets maxPr_{\alpha} \times mxPrs_{\beta}$
\State $sWgt_{\alpha \cup \beta} \gets sWgt_{\alpha} + sWgts_{\beta}$
\State $FUWSP(DB|{(\alpha \cup \beta))}, (\alpha \cup \beta),  maxPr_{\alpha \cup \beta}, \max(mxW_{\alpha}, sWgts_{\beta}),  sWgt_{\alpha \cup \beta},  |\alpha \cup \beta|)$
\EndIf
\EndFor
\EndProcedure
\Statex
\end{algorithmic}
\label{algo:fuws}
\end{algorithm}

% InUSP
\subsection{InUSP}
\label{subsec:inusp-pseudo-code}

\makeatletter
\renewcommand{\ALG@beginalgorithmic}{\small}
\makeatother
\algrenewcommand{\alglinenumber}{\small}
\makeatletter
\renewcommand{\ALG@beginalgorithmic}{\small}
\makeatother
\algrenewcommand{\alglinenumber}{\small}
\begin{algorithm}[htb] 
\caption{Procedure of \textit{uWSInc+}}
\begin{algorithmic}[1] 
\Statex
\Require \textit{DB:} initial database,  $\Delta {DB}$ : new increments,  \textit{min\_sup:} minimum support threshold,  $\mu$: buffer ratio,  \textit{wgt\_fct:} weight factor%\newline
\Ensure \textit{FS:} set of frequent patterns %\textit{SFS: } the set of semi-frequent patterns \newline
\Statex
\Procedure{InitialMining}{$DB$,  $\Delta{DB}_{i}$,  \textit{min\_sup},  $\mu$, \textit{wgt\_fct}}
% \State $minExpSup \gets$  \textit{min\_Sup}$\times uSDBsize$ 
% \State
\State $seqTrie \gets FUWS(DB,  min\_sup \times \mu, \textit{wgt\_fct})$
\State $pfsTrie \gets\ Trie\ to\ store\ PFS\ which\ is\ initialized\ as\ empty$
% \Comment{All FS and SFS stored into a trie}
% \State $triePFS \gets \textit{Dynamic Trie for Possible-frequent sequences after increments}$
\ForAll{$\Delta{DB}_{i}$}
\State $DBSize\gets DBSize + \Delta{DB}_{i}Size $
\State $seqTrie$, $pfsTrie$ $\gets$ uWSInc+($\Delta{DB}_{i}$,  $min\_sup$,  $\mu$, \textit{wgt\_fct}, $seqTrie$, $pfsTrie$)
\EndFor
\EndProcedure                                                
\Statex

\Procedure{uWSInc+}{$\Delta{DB}_{i}$,  $min\_sup$,  $\mu$, \textit{wgt\_fct}, $seqTrie$, $pfsTrie$}
\State $LWES = 2 \times min\_Sup \times \mu \times \Delta{DB}_{i}Size \times WAM^{'} \times wgt\_fct$ \Comment{choice of \textit{LWES} may vary}
\State $lfsTrie \gets FUWS(\Delta{DB}_{i},  2 \times min\_Sup \times \mu, \textit{wgt\_fct})$
% \ForAll{$S \in \Delta{DB}_{i}$}
% % \State $seqTrie.update\_support(S)$ \Comment{ $\forall x: Update Support(x),  x \in (FS \lor SFS) $}
% \State Update wExpSup($\alpha$) for S where $\alpha \in (FS \lor SFS)$ and stored into \textit{seqTrie}
% \State Update wExpSup($\beta$) for S where $\beta \in (PFS)$ and stored into \textit{pfsTrie}
% \EndFor
\State \textbf{Call} SupCalc($\Delta {DB}_{i}$,  \textit{seqTrie})
\State \textbf{Call} SupCalc($\Delta {DB}_{i}$,  \textit{pfsTrie})
\State $minWES \gets min\_sup \times DBsize \times WAM \times wgt\_fct$
% \ForAll{$S \in \Delta{DB}_{i}$}
% \State $pfsTrie.update\_support(S)$ \Comment{ $\forall x: Update Support(x),  x \in (PFS) $}
% \EndFor

% \State $pfsTrie \gets pfsTrie.merge\_with(lfsTrie)$ 
% \State $seqTrie \gets seqTrie.merge\_with(pfsTrie)$ 
% \State $seqTrie.update(\textit{semiWExpSup})$ \Comment{$\exists x,   Support(x)<semiWExpSup:Delete Node(x)$}
\ForAll{$\alpha \in (FS \lor SFS)$ stored into \textit{seqTrie}}
\If{$wExpSup(\alpha) < (minWES \times \mu $)}
\State Delete pattern $\alpha$ from \textit{seqTrie}
\If{$wExpSup(\alpha) \geq LWES $}
\State Insert pattern $\alpha$ into \textit{pfsTrie}
\EndIf
\EndIf
\EndFor
\ForAll{$\beta \in PFS$ stored into \textit{pfsTrie}}
\If{$wExpSup(\beta) \geq (minWES \times \mu)$}
\State Delete pattern $\beta$ from \textit{pfsTrie}
\State Insert pattern $\beta$ into \textit{seqTrie}
\ElsIf{$wExpSup(\beta) < LWES)$}
\State Delete pattern $\beta$ from \textit{pfsTrie}
\EndIf
\EndFor
\ForAll{$\gamma \in LFS$ stored into \textit{lfsTrie}}
\If{$wExpSup(\gamma) \geq (minWES \times \mu)$ }
\State Insert $\gamma$ into \textit{seqTrie}
\ElsIf{$wExpSup(\gamma) \geq LWES)$ }
\State Insert $\gamma$ into \textit{pfsTrie}
\EndIf
\EndFor
% \State Remove patterns $\beta$ from \textit{pfsTrie} if $wExpSup(\beta) \geq ((minWES \times \mu) \lor  < LWES)$ 
% \State $pfsTrie.update(\textit{semiWExpSup},  localWExpSup )$ \Comment{$\exists x,   (Support(x) \geq semiWExpSup) \lor (Support(x) < localWExpSup ):Delete Node(x)$}
\State $FS \gets seqTrie.find\_frequent\_patterns(\textit{minWES})$
\EndProcedure
% \Statex
\end{algorithmic}
\label{algo:uWSInc+}
\end{algorithm}

\section*{Example Simulation}
\label{sec:simulation}
Let us consider Table  \ref{tab:initDB} as the initial database \textit{DB} and increments shown in Table \ref{tab:increments}.  For  this simulation,  support threshold,  min\_sup=20\%,  buffer ratio,  $\mu$=0.7 and wgt\_fct = 1.0. As a result,  the minimum weighted expected support threshold for frequent sequences,  \textit{minWES} = 1.05 and for semi-frequent sequences,  \textit{$minWES^{'} = 0.74$}. 

The detailed simulations of \textit{FUWS} on \textit{DB} in Table  \ref{tab:initDB} has been shown in Figure  \ref{fig:fuws_simulation} where we compared the value of $wExpSup^{cap}$ for a sequence with $minWES^{'}$ to find out the candidates of frequent and semi-frequent sequences together. The semi-frequent sequences will be used in our incremental techniques later.

\begin{figure}[tbhp] 
    \centering
    \includegraphics[width=\linewidth]{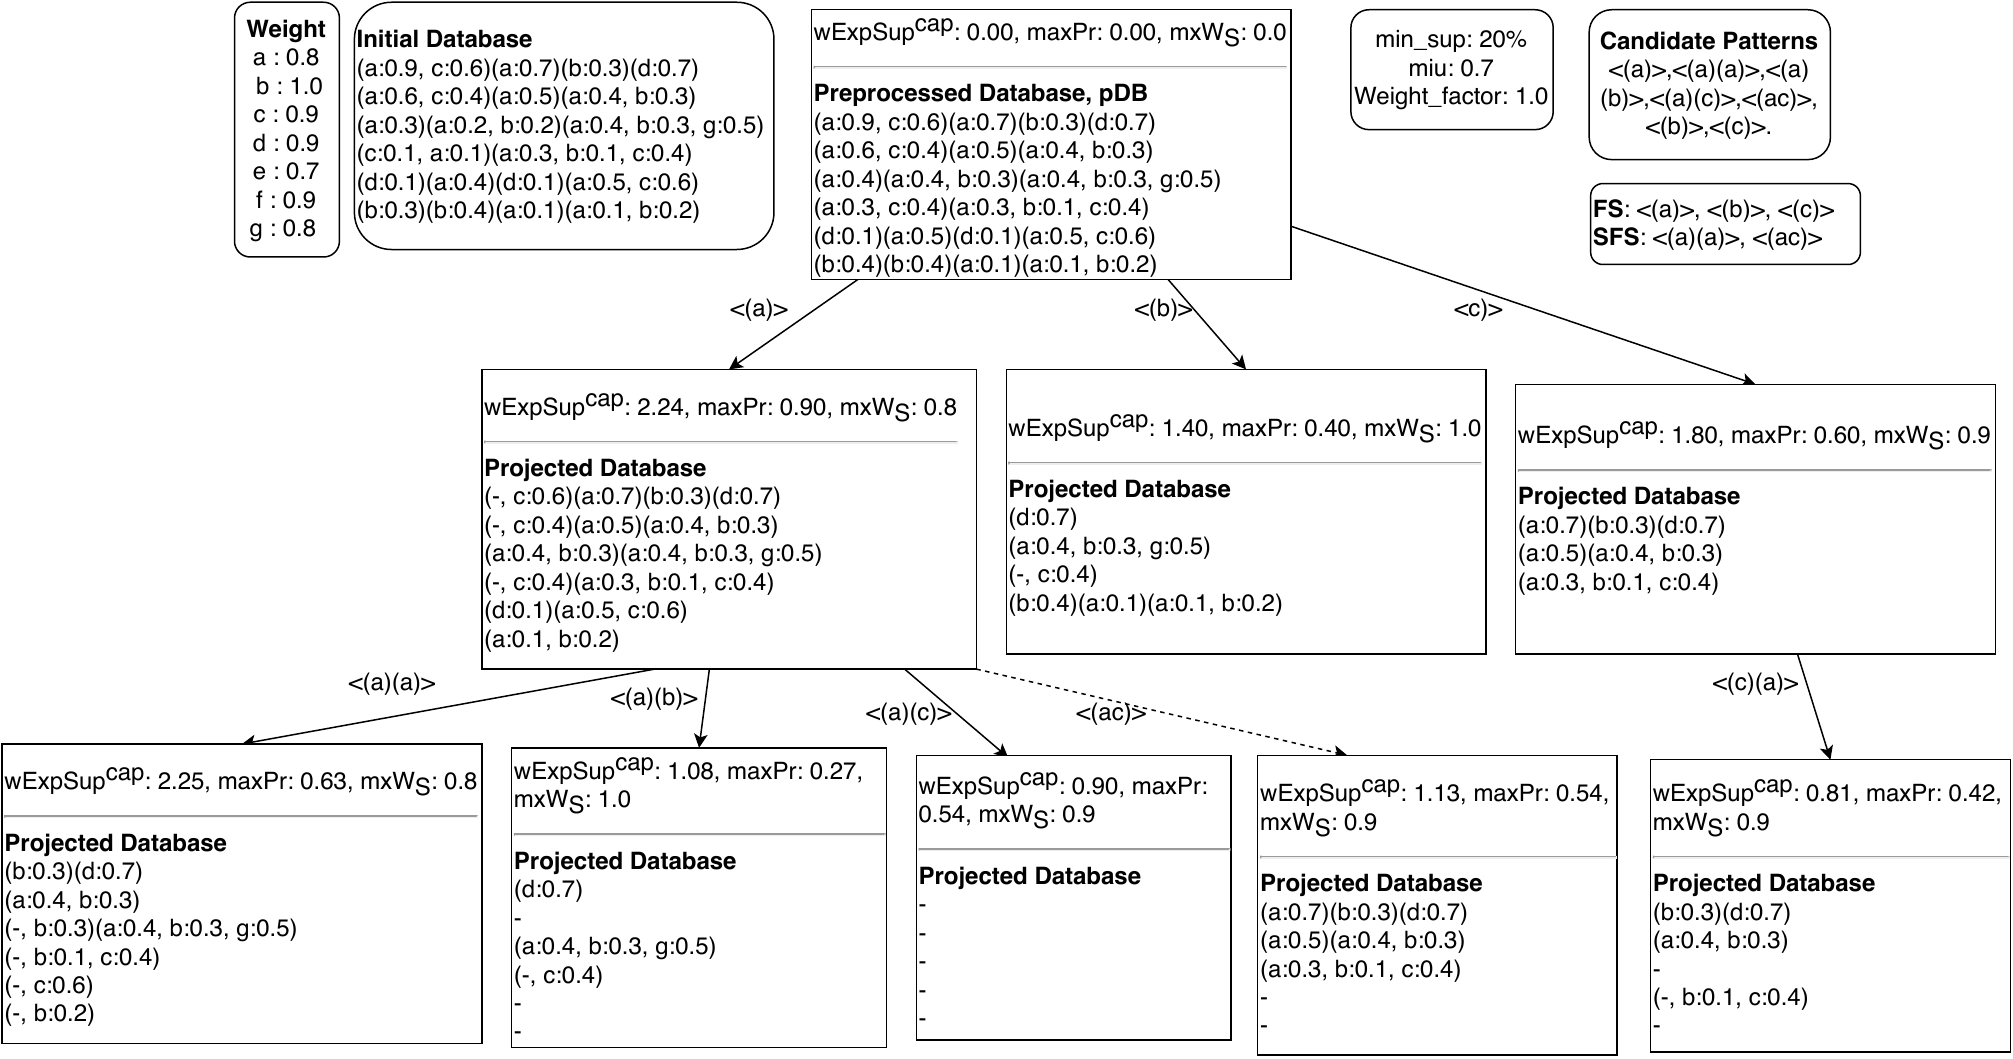}
			\caption{FUWS simulation for Initial Database, DB in Table \ref{tab:initDB}}
			\label{fig:fuws_simulation}
\end{figure}

% \begin{table}[tbh!]
% \centering
% \begin{tabular}{cc}
% \hline
% \multicolumn{1}{c}{\textbf{Id}} & \multicolumn{1}{c}{\textbf{Preprocessed Sequence}}              \\ \hline
% 1 & (a:0.9)(c:0.6)(a:0.9)(b:0.3)(d:0.9 \\ 
% 2 & (a:0.9,  c:0.4)(a:0.9)(a:0.8,  c:0.3) \\ 
% 3 & (a:0.3)(a:0.2,  b:0.2)(a:0.2,  b:0.1,  g:0.5)  \\
% 4 & (a:0.4,  c:0.5)(a:0.3,  b:0.1,  c:0.5)   \\ 
% 5 & (c:0.3)(a:0.9)(d:0.1)(a:0.6,  c:0.1) \\
% 6 & (b:0.4)(b:0.4)(a:0.1)(a:0.1,  b:0.2)   \\ \hline
% \end{tabular}%
% \caption{Preprocessed Database,  $pSDB$}
% \label{tab:prepocessed}
% \end{table}

\textit{FUWS} algorithm processes \textit{DB} in the way that has been described in Algorithm \ref{algo:fuws}. The preprocessed database has been shown as \textit{pDB} in Figure \ref{fig:fuws_simulation}. The \textit{FUWS} algorithm uses \textit{pDB} to find the potential candidates. An item is called s-extendable (or i-extendable) when the the value of $wExpSup^{cap}$ for the sequence extension (or itemset extension) of a prefix by that item satisfies the threshold $minWES^{'}$. First of all, it finds out extendable items considering the prefix pattern which is empty initially. Thus the resulting super sequences  are $\textless{}(a)\textgreater{} : 2.24, \textless{}(b)\textgreater{} : 1.40, \textless{}(c)\textgreater{} : 1.80$ where the real numbers associated with each item denotes the value of $wExpSup^{cap}$ for the respective super patterns. It projects the database recursively while considering newly generated super pattern as prefix pattern and finds out extendable items following the same process. In Figure \ref{fig:fuws_simulation}, an edge label indicates an extendable item and the edge type indicates the extension type such that solid lines are for s-extensions and dashed lines are for i-extensions. In this example, \textit{FUWS} algorithm considers $\textless{}(a)\textgreater{}$ as first prefix pattern and it projects \textit{pDB} accordingly. After that,  the algorithm finds i-extendable items which is $\textless{}(\_c)\textgreater{}$ and s-extendable items for the prefix pattern $\textless{}(a)\textgreater{}$ which are $\textless{}(a)\textgreater{}, \textless{}(b)\textgreater{}$ and $\textless{}(c)\textgreater{}$. Consequently, newly generated super patterns are $\textless{}(a)(a)\textgreater{}:2.25, \textless{}(a)(b)\textgreater{}:1.08, \textless{}(a)(c)\textgreater{}:0.90$ and $\textless{}(ac)\textgreater{}:1.13$. Then again it considers each super patterns as prefix pattern individually and tries to find out longer patterns by following the same process recursively.  In this example, as the algorithm does not find any extendable item for these patterns, so it backtracks to project the database considering $\textless{}(b)\textgreater{}$ as next 1-length prefix pattern. Again, there is no extendable items for $\textless{}(b)\textgreater{}$. Then it takes $\textless{}(c)\textgreater{}$ as next prefix pattern and finds out only one extendable item which is $\textless{}(a)\textgreater{}$. The algorithm repeats the same process for $\textless{}(c)(a)\textgreater{}$. Also no extendable items are found for prefix pattern $\textless{}(c)(a)\textgreater{}$. As there is no unexplored patterns, the recursive process terminates. It stores all potential candidate patterns into \textit{USeqTrie}.

To remove false positive patterns from candidate pattern set, the algorithm scans the database \textit{DB} to calculate the actual weighted expected support \textit{WES} for all candidates. Finally,  it finds out frequent and semi-frequent sequences by comparing the values of \textit{WES} with \textit{minWES} and \textit{$minWES^{'}$}. The resultant \textit{FS}: $\textless{}(a)\textgreater{}:2.24,\textless{}(b)\textgreater{}:1.4,\textless{}(c)\textgreater{}:1.8$ and \textit{SFS}: $\textless{}(a)(a)\textgreater{}:1.03,  \textless{}(a, c)\textgreater{}:1.02$.

\begin{table}[h]
    \centering
    % \small
    \begin{tabular}{|c|c|l|}
        \hline
        \textbf{Increment} & \textbf{Id} &      \textbf{Sequence} \\ \hline \hline

        \multirow{4}{*}{$\Delta DB_{1}$}
        &
          7 &  (c:0.6, a:0.7)(a: 0.8)(f:0.9, a:0.6)            \\ \cline{2-3}
        & 8 & (c:0.6, a:0.4)(c:0.8)(a:0.6)(f:0.5)(g:0.4, c:0.7) \\ \cline{2-3}
        & 9 & (f:0.8)(a:0.3)(c:0.9)(d:0.9)(f:0.5, a:0.7, d:0.4)  \\ \cline{2-3}
        & 10 & (c:0.7)(a:0.1)(a:0.8, c:0.6, d:0.8) \\ \hline \hline 
        \multirow{3}{*}{ $\Delta DB_{2}$ }
        &
          11 & (f:0.1)(f:0.3, c:0.7)(a:0.9)(d:0.9)(f:0.2, g:0.1) \\ \cline{2-3}
        & 12 & (a:0.2, c:0.1)(b:0.8)(f:0.4, e:0.4)(g:0.1)(e:0.5, g:0.2)    \\ \cline{2-3}
        & 13 & (c:0.6)(a:0.9)(d:0.6)(e:0.6)(a:0.5, e:0.4, c:0.1)\\ \hline
    \end{tabular}
    \caption{Increments,  $\Delta DB_{i}$}
    \label{tab:increments}
\end{table}

\begin{table}[h]
    \centering
    % \small
    \begin{tabular}{|c|c|l|c|l|}
    \hline
    \textbf{Inc.} & \multicolumn{2}{|c|}{\textbf{uWSInc}} & \multicolumn{2}{|c|}{\textbf{uWSInc+}} \\ \hline 
    
    \multirow{7}{*}{ $\Delta DB_{1}$ } & \multirow{5}{*}{FS:}  & $<(a)> : 4.56$ & \multirow{3}{*}{LFS:} & $<(a)>:2.32, <(c)>:2.7, <(d)>:1.53, <(f)>:1.98,$\\ 
            
    & & $<(a)(a)> : 1.90$ & & $<(a)(f)>:0.99, <(ac)>:0.97, <(c)(a)>:1.83,$ \\         
    
    & & $<(a, c)> : 1.99$  & & $ <(c)(f)>:1.23, <(f)(c)>:0.96$ \\ \cline{4-5}
    
    & & $<(c)> : 4.50$ & \multirow{2}{*}{FS:} & $<(a)> : 4.56, <(a)(a)> : 1.9, <(a,c)> : 1.99,$\\
    
    & & & & $<(c)> : 4.50, <(c)(a)> : 1.83, <(f)> : 1.98$ \\ \cline{2-5}
    
    & \multirow{2}{*}{SFS:} & \multirow{2}{*}{$<(c)(a)>:1.4$} & SFS: & $<(c)(d)>:1.23,<(b)>:1.4,<(c)(f)>:1.25,<(d)>:1.53$  \\ \cline{4-5}
    
    & & & PFS: & $<(a)(f)>:0.99, <(f)(c)>:0.96$ \\ \hline \hline

    \multirow{8}{*}{ $\Delta DB_{2}$ } & \multirow{5}{*}{FS:}  &   & \multirow{3}{*}{LFS:} &  $<(a)>:1.6, <(a)(d)>:1.15, <(b)>:0.8, <(c)>:1.26,$ \\ 
            
    & & $<(a)> : 6.16$ & & $<(d)>:1.35, <(c)(d)>:0.89, <(c)(a)>:1.99, $ \\        
    
     & & $<(a)(a)> : 2.26$ & & $<(c)(a)(d)>:0.77,<(e)>:0.77$ \\ \cline{4-5}
    
    & & $<(c)> : 5.76$ & \multirow{2}{*}{FS:} & $<(a)>:6.16, <(a)(a)>:2.26, <(c)>:5.76,$ \\
    
    & &  &  & $<(c)(a)>:2.82, <(d)>:2.88, <(f)>:2.61$ \\ \cline{2-5}
    
    & \multirow{3}{*}{SFS:} & $<(a, c)> : 2.05$ & SFS: &  $<(a, c)>:2.05, <(b)>:2.2, <(c)(d)>:2.12$ \\ \cline{4-5}
    
    &  & $<(b)> : 2.20$ & \multirow{2}{*}{PFS:}  & $<(a)(d)>:1.15, <(c)(f)>:1.41, <(a)(f)>:1.22,$\\ 
    
    & & &  & $<(e)>:0.77, <(f)(c)>:1.03, <(c)(a)(d)>:0.77$ \\ \hline

    \iffalse 
    \multirow{}{}
    \begin{tabular}{c}
     $\Delta DB_{2}$
     \end{tabular}
     &
    &
    \begin{tabular}{ll}
    SFS: &       
    \begin{tabular}{l}
    
    \end{tabular}    \\ \hline
    PFS: &
    \begin{tabular}{l}
     \\
    \end{tabular}    \\ 
    \end{tabular}%        
    \\ \hline  
    \fi 
    
    \end{tabular}%
    \caption{Simulation for Increments,  $\Delta DB_{i}$}
    \label{tab:increments_simulation}
\end{table}

After 1st increment,  $\Delta DB_{1}$,  the updated value of \textit{minWES}
is 1.74. The \textit{uWSInc} algorithm scans the $\Delta DB_{1}$ and updates the weighted expected support values for patterns in \textit{FS} and \textit{SFS} which are found in \textit{DB}. As a result,  \textit{FS} and \textit{SFS} are updated as shown in Table  \ref{tab:increments_simulation}. 
The second approach,  \textit{uWSInc+} runs \textit{FUWS} and finds the locally frequent set for
$\Delta DB_{1}$,  \textit{LFS},  using 0.96 as \textit{LWES}. Users can set different local threshold \textit{LWES} based on the size and nature of increments,  distribution of items,  etc. In this simulation, let us assume that $LWES = 2\times min\_sup \times |\Delta DB_{i}| \times WAM \times \mu \times wgt\_fct $ for $\Delta DB_{i}$. By scanning $\Delta DB_{1}$,  it updates the WES for \textit{FS},  \textit{SFS},  and \textit{PFS} which are found in initial database \textit{DB}. After that \textit{FS},  \textit{SFS} and \textit{PFS} have been updated according to the updated \textit{minWES} and \textit{LWES}. The results are shown in Table  \ref{tab:increments_simulation}. From Table  \ref{tab:increments_simulation},  we can see that new pattern \textless{}(c)(a)\textgreater{} and \textless{}(f)\textgreater{} appear in \textit{FS} and $<(b)>$, \textless{}(d)\textgreater{}, \textless{}(c)(d)\textgreater{} and \textless{}(c)(f)\textgreater{} appear in \textit{SFS} of \textit{uWSInc+} but not in \textit{uWSInc}. This pattern \textless{}(d)\textgreater{}, \textless{}(c)(d)\textgreater{} and \textless{}(c)(f)\textgreater{} might be frequent later after few increments. The \textit{uWSInc+} might be able to find them which \textit{uWSInc} could never do.

Similarly for the second increment $\Delta DB_{2}$,  the \textit{uWSInc} and \textit{uWSInc+} algorithms use \textit{FS},  \textit{SFS},  and \textit{PFS} which are updated after 1st increment and  follow the same process to generate new \textit{FS},  \textit{SFS},  and \textit{PFS}.  The results are shown in Table  \ref{tab:increments_simulation}. Finally, we can see that two patterns  \textless{}(c)(a)\textgreater{}, \textless{}(d)\textgreater{} and \textless{}(f)\textgreater{},  have become frequent after this increment  which are found by \textit{uWSInc+} but not \textit{uWSInc}. This makes the difference between our two approaches clear as \textit{uWSInc+} can find them but \textit{uWSInc} cannot.
